# Supplementary material for: Scale setting of SU($N$) Yang--Mills theory, topology and large-$N$ volume independence
Source: arXiv:2511.07355 ancillary file (2026-03-27)
Supplement: Supplementary file 1 [file supplemental_material.pdf]

# Scale setting of SU($N$) Yang–Mills theory, topology and large-$N$ volume independence

Claudio Bonanno, Jorge Luis Dasilva Golán,
Massimo D'Elia, Margarita García Pérez, Andrea Giorgieri

# SUPPLEMENTAL MATERIAL

## Contents

**1 Finite-volume scales** **1**
1.1 Defined from $\varphi(t)$ . . . . . . 1
1.1.1 Unimproved . . . . . . 1
1.1.2 Improved . . . . . . 4
1.2 Defined from $\varphi'(t)$ . . . . . . 7
1.2.1 Unimproved . . . . . . 7
1.2.2 Improved . . . . . . 10

**2 Infinite-volume scales** **13**
2.1 $N$-by-$N$ fit strategy . . . . . . 13
2.1.1 With and without topological projection . . . . . . 13
2.1.2 Combined final results . . . . . . 16
2.2 Global fit strategy . . . . . . 17
2.2.1 With and without topological projection . . . . . . 17
2.2.2 Combined final results . . . . . . 20

**3 Continuum scale ratios** **21**
3.1 $N$-by-$N$ fit strategy . . . . . . 21
3.2 Global fit strategy . . . . . . 21

# 1 Finite-volume scales

## 1.1 Defined from $\varphi(t)$

### 1.1.1 Unimproved

| $N = 3$, Unimproved | | | | | | | | |
|---|---|---|---|---|---|---|---|---|
| | | | Any $Q$ | | | $Q = 0$ | | |
| $b$ | $L_s$ | $L$ | $t_0/a^2$ | $t_1/a^2$ | $w_0^2/a^2$ | $t_0/a^2$ | $t_1/a^2$ | $w_0^2/a^2$ |
| 0.35883 | 16 | 24 | 12.681(44) | 5.344(11) | 13.235(75) | 13.762(67) | 5.551(16) | 15.38(15) |
| | | 30 | 12.312(43) | 5.266(12) | 12.619(72) | 12.836(67) | 5.375(17) | 13.52(12) |
| | | 36 | 12.215(21) | 5.2424(62) | 12.483(35) | 12.491(49) | 5.300(12) | 12.947(80) |
| | 20 | 24 | 12.568(36) | 5.3172(87) | 13.063(60) | 13.190(55) | 5.440(12) | 14.22(11) |
| | | 30 | 12.454(26) | 5.2940(64) | 12.859(43) | 12.769(42) | 5.356(10) | 13.413(72) |
| | | 36 | 12.454(24) | 5.2949(65) | 12.852(39) | 12.663(46) | 5.339(12) | 13.214(77) |
| | 24 | 24 | 12.593(21) | 5.3220(54) | 13.098(37) | 13.015(46) | 5.408(12) | 13.862(83) |
| | | 30 | 12.509(26) | 5.3039(59) | 12.953(42) | 12.769(43) | 5.360(11) | 13.392(75) |
| | | 36 | 12.493(24) | 5.3015(67) | 12.928(39) | 12.661(44) | 5.339(12) | 13.192(74) |
| 0.37583 | 18 | 38 | 26.53(34) | 11.43(11) | 27.06(54) | 28.89(60) | 11.86(16) | 31.6(1.2) |
| | | 46 | 26.64(18) | 11.435(57) | 27.29(30) | 27.53(25) | 11.618(68) | 28.83(43) |
| | | 54 | 26.06(16) | 11.304(45) | 26.37(24) | 26.88(22) | 11.462(59) | 27.79(36) |
| | 24 | 38 | 27.79(24) | 11.776(67) | 28.70(38) | 29.31(47) | 12.08(11) | 31.52(88) |
| | | 46 | 27.60(19) | 11.724(50) | 28.47(31) | 28.73(26) | 11.984(64) | 30.33(46) |
| | | 54 | 27.30(12) | 11.658(31) | 27.95(19) | 28.13(21) | 11.845(62) | 29.37(35) |
| | 30 | 38 | 28.51(16) | 11.947(43) | 29.86(28) | 29.34(27) | 12.103(68) | 31.40(51) |
| | | 46 | 28.37(19) | 11.901(52) | 29.54(32) | 28.68(22) | 11.959(60) | 30.08(38) |
| | | 54 | 27.72(22) | 11.728(64) | 28.65(37) | 28.26(41) | 11.829(99) | 29.56(70) |
| 0.38844 | 24 | 50 | 49.38(65) | 20.69(15) | 52.2(1.1) | 52.54(73) | 21.34(14) | 58.2(1.6) |
| | | 60 | 47.30(38) | 20.31(11) | 48.32(64) | 49.33(64) | 20.71(21) | 51.7(1.1) |
| | 32 | 50 | 51.1(2.2) | 21.11(72) | 54.8(3.8) | 52.7(3.1) | 21.47(84) | 57.7(5.0) |
| | | 60 | 49.55(35) | 21.02(11) | 51.10(58) | 50.28(58) | 21.18(16) | 52.4(1.0) |

Table 1: SU(3) finite-volume scale-setting results with TBCs and no improvement, with and without projection onto the $Q = 0$ topological sector.

| $N = 5$, Unimproved | | | | | | | | |
|---|---|---|---|---|---|---|---|---|
| | | | Any $Q$ | | | $Q = 0$ | | |
| $b$ | $L_s$ | $L$ | $t_0/a^2$ | $t_1/a^2$ | $w_0^2/a^2$ | $t_0/a^2$ | $t_1/a^2$ | $w_0^2/a^2$ |
| 0.35971 | 12 | 18 | 6.6173(60) | 2.7433(14) | 7.044(11) | 6.7484(89) | 2.7687(20) | 7.298(18) |
| | | 22 | 6.5936(82) | 2.7396(19) | 6.995(15) | 6.679(15) | 2.7566(34) | 7.158(27) |
| | | 26 | 6.5818(55) | 2.7364(14) | 6.9797(99) | 6.637(11) | 2.7471(25) | 7.081(21) |
| | 14 | 18 | 6.6485(87) | 2.7493(20) | 7.103(17) | 6.749(12) | 2.7696(32) | 7.293(27) |
| | | 22 | 6.6319(80) | 2.7461(19) | 7.073(15) | 6.684(13) | 2.7572(33) | 7.168(23) |
| | | 26 | 6.6237(62) | 2.7444(16) | 7.055(11) | 6.6679(99) | 2.7526(23) | 7.140(18) |
| | 16 | 18 | 6.6418(56) | 2.7470(14) | 7.097(10) | 6.710(15) | 2.7595(32) | 7.235(27) |
| | | 22 | 6.6149(67) | 2.7415(15) | 7.048(12) | 6.6792(88) | 2.7531(21) | 7.171(16) |
| | | 26 | 6.6278(53) | 2.7446(15) | 7.0701(97) | 6.655(13) | 2.7487(32) | 7.129(25) |
| 0.37504 | 14 | 28 | 14.331(42) | 5.944(11) | 15.212(74) | 14.735(56) | 6.020(14) | 15.99(11) |
| | | 34 | 14.319(50) | 5.937(13) | 15.194(90) | 14.607(67) | 5.989(16) | 15.75(13) |
| | | 40 | 14.310(36) | 5.930(11) | 15.217(64) | 14.472(51) | 5.962(13) | 15.517(93) |
| | 18 | 28 | 14.615(52) | 6.002(11) | 15.676(95) | 14.877(36) | 6.0517(92) | 16.188(71) |
| | | 34 | 14.566(35) | 5.9984(87) | 15.547(63) | 14.640(70) | 6.010(16) | 15.72(13) |
| | | 40 | 14.504(24) | 5.9784(64) | 15.472(43) | 14.570(46) | 5.994(11) | 15.587(86) |
| | 22 | 28 | 14.741(34) | 6.0295(89) | 15.877(64) | 14.896(49) | 6.063(13) | 16.151(97) |
| | | 34 | 14.596(32) | 5.9997(89) | 15.605(61) | 14.69(11) | 6.008(25) | 15.83(20) |
| | | 40 | 14.654(25) | 6.0118(57) | 15.716(46) | 14.666(52) | 6.007(14) | 15.778(98) |
| 0.38683 | 28 | 38 | – | – | – | 26.331(57) | 10.703(14) | 28.58(11) |
| | | 42 | – | – | – | 26.366(57) | 10.718(14) | 28.57(11) |
| | | 46 | – | – | – | 26.252(49) | 10.704(12) | 28.321(92) |

Table 2: SU(5) finite-volume scale-setting results with TBCs and no improvement, with and without projection onto the $Q = 0$ topological sector. Empty cells correspond to simulation points for which we were not able to use the PTBC algorithm to sample $Q$ correctly.

| $N = 8$, Unimproved | | | | | | | | |
|---|---|---|---|---|---|---|---|---|
| | | | Any $Q$ | | | $Q = 0$ | | |
| $b$ | $L_s$ | $L$ | $t_0/a^2$ | $t_1/a^2$ | $w_0^2/a^2$ | $t_0/a^2$ | $t_1/a^2$ | $w_0^2/a^2$ |
| 0.35867 | 6 | 14 | 4.5504(70) | 1.8734(15) | 4.905(13) | 4.6349(55) | 1.8886(12) | 5.078(11) |
| | | 16 | 4.4975(50) | 1.8627(13) | 4.8094(97) | 4.5709(41) | 1.8766(11) | 4.9530(93) |
| | | 18 | 4.4960(36) | 1.86231(80) | 4.8070(65) | 4.5593(49) | 1.8745(11) | 4.9282(93) |
| | 8 | 14 | 4.5575(41) | 1.88124(89) | 4.8947(77) | 4.6239(48) | 1.8931(24) | 5.0289(97) |
| | | 16 | 4.5452(33) | 1.87876(84) | 4.8730(61) | 4.5876(44) | 1.8867(11) | 4.9560(84) |
| | | 18 | 4.5467(22) | 1.87905(55) | 4.8752(42) | 4.5766(29) | 1.88451(80) | 4.9359(56) |
| | 10 | 14 | 4.5880(34) | 1.88784(70) | 4.9446(67) | 4.6268(65) | 1.8948(16) | 5.024(12) |
| | | 16 | 4.5761(36) | 1.88496(85) | 4.9245(70) | 4.6051(62) | 1.8911(14) | 4.980(12) |
| | | 18 | 4.5762(29) | 1.88505(94) | 4.9246(58) | 4.5937(50) | 1.8883(12) | 4.9613(93) |
| | 12 | 18 | 4.5864(32) | 1.88703(80) | 4.9441(61) | 4.6036(46) | 1.8900(12) | 4.9793(89) |
| 0.38352 | 12 | 28 | 17.27(12) | 6.998(28) | 18.83(23) | 17.48(15) | 7.041(33) | 19.26(30) |
| | | 32 | 17.219(53) | 6.989(13) | 18.74(10) | 17.299(56) | 7.001(15) | 18.93(11) |
| | | 36 | 17.170(36) | 6.9886(87) | 18.585(70) | 17.369(52) | 7.022(13) | 18.97(10) |
| | 16 | 28 | 17.330(59) | 7.040(14) | 18.86(11) | 17.412(70) | 7.056(18) | 19.01(14) |
| | | 32 | 17.347(49) | 7.040(13) | 18.885(97) | 17.420(62) | 7.053(14) | 19.04(13) |
| | | 36 | 17.329(36) | 7.0392(89) | 18.802(70) | 17.340(44) | 7.039(10) | 18.839(85) |
| | 20 | 28 | 17.60(12) | 7.092(26) | 19.27(23) | 17.64(14) | 7.102(29) | 19.35(27) |
| | | 32 | 17.376(63) | 7.049(15) | 18.91(12) | 17.420(68) | 7.057(18) | 18.99(13) |
| | | 36 | 17.436(45) | 7.060(11) | 18.978(86) | 17.431(45) | 7.058(11) | 18.977(86) |
| | 24 | 36 | 17.430(45) | 7.059(13) | 19.003(87) | 17.450(41) | 7.062(12) | 19.040(79) |
| 0.40008 | 36 | 48 | – | – | – | 39.06(15) | 15.768(36) | 42.69(33) |
| | | 54 | – | – | – | 39.128(98) | 15.797(24) | 42.72(19) |
| | | 60 | – | – | – | 39.120(90) | 15.790(23) | 42.74(18) |

Table 3: SU(8) finite-volume scale-setting results with TBCs and no improvement, with and without projection onto the $Q = 0$ topological sector. Empty cells correspond to simulation points for which we were not able to use the PTBC algorithm to sample $Q$ correctly.

### 1.1.2 Improved

| $N = 3$, Improved | | | | | | | | |
|---|---|---|---|---|---|---|---|---|
| | | | Any $Q$ | | | $Q = 0$ | | |
| $b$ | $L_s$ | $L$ | $t_0/a^2$ | $t_1/a^2$ | $w_0^2/a^2$ | $t_0/a^2$ | $t_1/a^2$ | $w_0^2/a^2$ |
| 0.35883 | 16 | 24 | 12.631(44) | 5.277(11) | 13.253(76) | 13.710(67) | 5.482(16) | 15.41(15) |
| | | 30 | 12.261(43) | 5.202(12) | 12.614(72) | 12.783(66) | 5.309(16) | 13.52(12) |
| | | 36 | 12.167(21) | 5.1791(61) | 12.478(35) | 12.441(48) | 5.236(12) | 12.943(80) |
| | 20 | 24 | 12.521(36) | 5.2512(86) | 13.080(60) | 13.142(55) | 5.372(12) | 14.25(11) |
| | | 30 | 12.404(26) | 5.2300(64) | 12.852(43) | 12.718(42) | 5.291(10) | 13.408(72) |
| | | 36 | 12.407(24) | 5.2313(65) | 12.844(39) | 12.615(46) | 5.275(12) | 13.206(77) |
| | 24 | 24 | 12.548(21) | 5.2555(54) | 13.117(37) | 12.969(46) | 5.340(12) | 13.886(84) |
| | | 30 | 12.461(25) | 5.2394(59) | 12.949(42) | 12.720(43) | 5.294(11) | 13.388(76) |
| | | 36 | 12.447(24) | 5.2374(66) | 12.922(39) | 12.615(44) | 5.275(12) | 13.186(73) |
| 0.37583 | 18 | 38 | 26.48(34) | 11.36(11) | 27.07(54) | 28.84(60) | 11.79(16) | 31.6(1.2) |
| | | 46 | 26.59(18) | 11.368(57) | 27.28(30) | 27.48(25) | 11.550(68) | 28.83(43) |
| | | 54 | 26.01(16) | 11.238(45) | 26.37(24) | 26.83(22) | 11.395(59) | 27.79(36) |
| | 24 | 38 | 27.73(24) | 11.711(66) | 28.71(38) | 29.25(47) | 12.01(11) | 31.54(88) |
| | | 46 | 27.55(19) | 11.660(50) | 28.47(31) | 28.68(26) | 11.920(63) | 30.33(46) |
| | | 54 | 27.25(12) | 11.595(31) | 27.95(19) | 28.08(21) | 11.781(62) | 29.37(35) |
| | 30 | 38 | 28.46(16) | 11.881(42) | 29.88(28) | 29.29(27) | 12.036(67) | 31.42(51) |
| | | 46 | 28.32(19) | 11.836(51) | 29.54(32) | 28.63(22) | 11.894(60) | 30.08(38) |
| | | 54 | 27.68(22) | 11.664(63) | 28.64(37) | 28.22(41) | 11.765(99) | 29.55(70) |
| 0.38844 | 24 | 50 | 49.32(65) | 20.62(15) | 52.2(1.1) | 52.48(73) | 21.27(14) | 58.2(1.6) |
| | | 60 | 47.25(38) | 20.25(11) | 48.32(64) | 49.28(64) | 20.64(21) | 51.7(1.1) |
| | 32 | 50 | 51.1(2.2) | 21.05(72) | 54.8(3.8) | 52.7(3.1) | 21.41(84) | 57.7(5.0) |
| | | 60 | 49.50(35) | 20.95(11) | 51.09(58) | 50.23(58) | 21.12(16) | 52.4(1.0) |

Table 4: SU(3) finite-volume scale-setting results with TBCs and improvement of lattice artifacts, with and without projection onto the $Q = 0$ topological sector.

| $N = 5$, Improved | | | | | | | | |
|---|---|---|---|---|---|---|---|---|
| | | | Any $Q$ | | | $Q = 0$ | | |
| $b$ | $L_s$ | $L$ | $t_0/a^2$ | $t_1/a^2$ | $w_0^2/a^2$ | $t_0/a^2$ | $t_1/a^2$ | $w_0^2/a^2$ |
| | | 18 | 6.5680(60) | 2.6748(14) | 7.066(11) | 6.6987(89) | 2.6996(19) | 7.323(18) |
| | 12 | 22 | 6.5427(82) | 2.6725(19) | 6.995(15) | 6.627(15) | 2.6892(33) | 7.158(27) |
| | | 26 | 6.5331(55) | 2.6698(14) | 6.9772(99) | 6.588(11) | 2.6802(25) | 7.079(21) |
| | | 18 | 6.5997(87) | 2.6807(20) | 7.125(17) | 6.700(12) | 2.7005(32) | 7.317(27) |
| 0.35971 | 14 | 22 | 6.5812(79) | 2.6789(19) | 7.072(15) | 6.633(12) | 2.6898(33) | 7.168(23) |
| | | 26 | 6.5751(62) | 2.6776(16) | 7.052(11) | 6.6190(98) | 2.6857(23) | 7.136(18) |
| | | 18 | 6.5936(56) | 2.6783(14) | 7.119(11) | 6.662(15) | 2.6905(32) | 7.259(28) |
| | 16 | 22 | 6.5648(67) | 2.6743(15) | 7.047(12) | 6.6286(87) | 2.6856(21) | 7.171(17) |
| | | 26 | 6.5797(53) | 2.6778(15) | 7.0666(97) | 6.607(13) | 2.6817(32) | 7.126(25) |
| | | 28 | 14.280(42) | 5.877(11) | 15.226(74) | 14.684(56) | 5.951(14) | 16.01(11) |
| | 14 | 34 | 14.269(50) | 5.871(13) | 15.193(91) | 14.556(67) | 5.922(16) | 15.75(13) |
| | | 40 | 14.263(36) | 5.864(11) | 15.217(64) | 14.423(51) | 5.895(12) | 15.516(93) |
| | | 28 | 14.565(52) | 5.934(11) | 15.693(95) | 14.826(36) | 5.9838(91) | 16.208(72) |
| 0.37504 | 18 | 34 | 14.515(35) | 5.9321(86) | 15.545(63) | 14.590(70) | 5.944(16) | 15.72(13) |
| | | 40 | 14.456(24) | 5.9124(63) | 15.470(43) | 14.521(46) | 5.928(11) | 15.585(86) |
| | | 28 | 14.691(34) | 5.9618(89) | 15.894(64) | 14.845(49) | 5.995(13) | 16.170(97) |
| | 22 | 34 | 14.546(32) | 5.9332(89) | 15.602(61) | 14.64(11) | 5.941(25) | 15.83(20) |
| | | 40 | 14.606(25) | 5.9455(57) | 15.712(46) | 14.618(52) | 5.941(14) | 15.774(98) |
| | | 38 | – | – | – | 26.281(57) | 10.636(14) | 28.60(11) |
| 0.38683 | 28 | 42 | – | – | – | 26.314(57) | 10.651(14) | 28.57(11) |
| | | 46 | – | – | – | 26.202(49) | 10.637(12) | 28.318(92) |

Table 5: SU(5) finite-volume scale-setting results with TBCs and improvement of lattice artifacts, with and without projection onto the $Q = 0$ topological sector. Empty cells correspond to simulation points for which we were not able to use the PTBC algorithm to sample $Q$ correctly.

| $N=8$, Improved | | | | | | | | |
|---|---|---|---|---|---|---|---|---|
| | | | Any $Q$ | | | $Q=0$ | | |
| $b$ | $L_s$ | $L$ | $t_0/a^2$ | $t_1/a^2$ | $w_0^2/a^2$ | $t_0/a^2$ | $t_1/a^2$ | $w_0^2/a^2$ |
| 0.35867 | 6 | 14 | 4.5042(70) | 1.8018(14) | 4.935(13) | 4.5885(55) | 1.8164(11) | 5.112(11) |
| | | 16 | 4.4468(50) | 1.7929(13) | 4.8221(99) | 4.5196(41) | 1.8063(11) | 4.9684(95) |
| | | 18 | 4.4454(35) | 1.79320(78) | 4.8081(65) | 4.5080(49) | 1.8049(11) | 4.9305(94) |
| | 8 | 14 | 4.5115(41) | 1.81006(86) | 4.9263(78) | 4.5778(48) | 1.8215(23) | 5.0629(99) |
| | | 16 | 4.4943(33) | 1.80916(82) | 4.8877(62) | 4.5363(44) | 1.8168(10) | 4.9724(86) |
| | | 18 | 4.4957(22) | 1.81009(54) | 4.8775(42) | 4.5253(29) | 1.81536(79) | 4.9389(56) |
| | 10 | 14 | 4.5421(34) | 1.81671(68) | 4.9767(68) | 4.5809(65) | 1.8234(16) | 5.057(13) |
| | | 16 | 4.5250(36) | 1.81540(83) | 4.9398(72) | 4.5538(61) | 1.8213(14) | 4.996(12) |
| | | 18 | 4.5249(29) | 1.81616(98) | 4.9269(58) | 4.5421(49) | 1.8193(12) | 4.9641(94) |
| | 12 | 18 | 4.5352(32) | 1.81807(78) | 4.9463(61) | 4.5521(46) | 1.8209(12) | 4.9819(90) |
| 0.38352 | 12 | 28 | 17.22(12) | 6.929(28) | 18.86(23) | 17.44(15) | 6.971(33) | 19.30(30) |
| | | 32 | 17.168(53) | 6.921(13) | 18.75(10) | 17.247(56) | 6.933(15) | 18.94(11) |
| | | 36 | 17.119(36) | 6.9209(86) | 18.585(71) | 17.318(52) | 6.954(12) | 18.98(10) |
| | 16 | 28 | 17.283(59) | 6.971(14) | 18.89(11) | 17.365(71) | 6.987(17) | 19.04(14) |
| | | 32 | 17.296(49) | 6.972(13) | 18.898(98) | 17.368(62) | 6.985(13) | 19.05(13) |
| | | 36 | 17.279(36) | 6.9717(89) | 18.803(70) | 17.290(44) | 6.971(10) | 18.840(85) |
| | 20 | 28 | 17.55(12) | 7.022(26) | 19.30(23) | 17.60(14) | 7.032(29) | 19.38(27) |
| | | 32 | 17.325(63) | 6.981(15) | 18.92(12) | 17.368(68) | 6.989(18) | 19.00(13) |
| | | 36 | 17.385(45) | 6.993(11) | 18.979(86) | 17.380(45) | 6.990(11) | 18.978(86) |
| | 24 | 36 | 17.379(45) | 6.992(13) | 19.003(87) | 17.399(41) | 6.995(12) | 19.041(79) |
| 0.40008 | 36 | 48 | – | – | – | 39.01(15) | 15.700(35) | 42.70(33) |
| | | 54 | – | – | – | 39.078(98) | 15.730(24) | 42.72(19) |
| | | 60 | – | – | – | 39.071(89) | 15.723(23) | 42.73(18) |

Table 6: SU(8) finite-volume scale-setting results with TBCs and improvement of lattice artifacts, with and without projection onto the $Q=0$ topological sector. Empty cells correspond to simulation points for which we were not able to use the PTBC algorithm to sample $Q$ correctly.

## 1.2 Defined from $\varphi'(t)$

### 1.2.1 Unimproved

| Primed, $N = 3$, Unimproved | | | | | | | | |
|---|---|---|---|---|---|---|---|---|
| | | | Any $Q$ | | | $Q = 0$ | | |
| $b$ | $L_s$ | $L$ | $t'_0/a^2$ | $t'_1/a^2$ | $w'^2_0/a^2$ | $t'_0/a^2$ | $t'_1/a^2$ | $w'^2_0/a^2$ |
| 0.35883 | 16 | 24 | 12.681(44) | 5.344(11) | 13.235(75) | 13.762(67) | 5.551(16) | 15.38(15) |
| | | 30 | 12.312(43) | 5.266(12) | 12.619(72) | 12.836(67) | 5.375(17) | 13.52(12) |
| | | 36 | 12.215(21) | 5.2424(62) | 12.483(35) | 12.491(49) | 5.300(12) | 12.947(80) |
| | 20 | 24 | 12.568(36) | 5.3172(87) | 13.063(60) | 13.190(55) | 5.440(12) | 14.22(11) |
| | | 30 | 12.454(26) | 5.2940(64) | 12.859(43) | 12.769(42) | 5.356(10) | 13.413(72) |
| | | 36 | 12.454(24) | 5.2949(65) | 12.852(39) | 12.663(46) | 5.339(12) | 13.214(77) |
| | 24 | 24 | 12.593(21) | 5.3220(54) | 13.098(37) | 13.015(46) | 5.408(12) | 13.862(83) |
| | | 30 | 12.509(26) | 5.3039(59) | 12.953(42) | 12.769(43) | 5.360(11) | 13.392(75) |
| | | 36 | 12.493(24) | 5.3015(67) | 12.928(39) | 12.661(44) | 5.339(12) | 13.192(74) |
| 0.37583 | 18 | 38 | 26.53(34) | 11.43(11) | 27.06(54) | 28.89(60) | 11.86(16) | 31.6(1.2) |
| | | 46 | 26.64(18) | 11.435(57) | 27.29(30) | 27.53(25) | 11.618(68) | 28.83(43) |
| | | 54 | 26.06(16) | 11.304(45) | 26.37(24) | 26.88(22) | 11.462(59) | 27.79(36) |
| | 24 | 38 | 27.79(24) | 11.776(67) | 28.70(38) | 29.31(47) | 12.08(11) | 31.52(88) |
| | | 46 | 27.60(19) | 11.724(50) | 28.47(31) | 28.73(26) | 11.984(64) | 30.33(46) |
| | | 54 | 27.30(12) | 11.658(31) | 27.95(19) | 28.13(21) | 11.845(62) | 29.37(35) |
| | 30 | 38 | 28.51(16) | 11.947(43) | 29.86(28) | 29.34(27) | 12.103(68) | 31.40(51) |
| | | 46 | 28.37(19) | 11.901(52) | 29.54(32) | 28.68(22) | 11.959(60) | 30.08(38) |
| | | 54 | 27.72(22) | 11.728(64) | 28.65(37) | 28.26(41) | 11.829(99) | 29.56(70) |
| 0.38844 | 24 | 50 | 49.38(65) | 20.69(15) | 52.2(1.1) | 52.54(73) | 21.34(14) | 58.2(1.6) |
| | | 60 | 47.30(38) | 20.31(11) | 48.32(64) | 49.33(64) | 20.71(21) | 51.7(1.1) |
| | 32 | 50 | 51.1(2.2) | 21.11(72) | 54.8(3.8) | 52.7(3.1) | 21.47(84) | 57.7(5.0) |
| | | 60 | 49.55(35) | 21.02(11) | 51.10(58) | 50.28(58) | 21.18(16) | 52.4(1.0) |

Table 7: SU(3) finite-volume scale-setting results with TBCs and no improvement, with and without projection onto the $Q = 0$ topological sector.

| Primed, $N = 5$, Unimproved | | | | | | | | |
|---|---|---|---|---|---|---|---|---|
| | | | Any $Q$ | | | $Q = 0$ | | |
| $b$ | $L_s$ | $L$ | $t'_0/a^2$ | $t'_1/a^2$ | $w'^2_0/a^2$ | $t'_0/a^2$ | $t'_1/a^2$ | $w'^2_0/a^2$ |
| 0.35971 | 12 | 18 | 6.0817(52) | 2.4300(12) | 6.6241(99) | 6.1938(77) | 2.4501(16) | 6.849(16) |
| | | 22 | 6.0618(72) | 2.4271(16) | 6.581(13) | 6.135(13) | 2.4408(28) | 6.725(25) |
| | | 26 | 6.0513(49) | 2.4246(11) | 6.5660(91) | 6.099(10) | 2.4329(20) | 6.657(19) |
| | 14 | 18 | 6.1085(76) | 2.4348(17) | 6.677(16) | 6.195(10) | 2.4509(26) | 6.846(24) |
| | | 22 | 6.0942(69) | 2.4322(16) | 6.650(13) | 6.139(11) | 2.4410(27) | 6.735(21) |
| | | 26 | 6.0873(55) | 2.4307(13) | 6.634(10) | 6.1251(86) | 2.4372(19) | 6.709(17) |
| | 16 | 18 | 6.1023(50) | 2.4328(12) | 6.6704(95) | 6.160(13) | 2.4427(27) | 6.793(25) |
| | | 22 | 6.0791(58) | 2.4284(12) | 6.627(11) | 6.1340(77) | 2.4375(17) | 6.737(15) |
| | | 26 | 6.0904(47) | 2.4310(12) | 6.6466(90) | 6.113(12) | 2.4341(26) | 6.699(24) |
| 0.37504 | 14 | 28 | 13.174(37) | 5.2613(95) | 14.308(68) | 13.519(49) | 5.320(12) | 15.004(99) |
| | | 34 | 13.164(45) | 5.255(10) | 14.295(83) | 13.409(58) | 5.296(13) | 14.79(11) |
| | | 40 | 13.154(32) | 5.2489(91) | 14.312(59) | 13.292(45) | 5.274(10) | 14.580(85) |
| | 18 | 28 | 13.422(45) | 5.3059(88) | 14.735(85) | 13.646(32) | 5.3456(75) | 15.189(65) |
| | | 34 | 13.383(31) | 5.3040(70) | 14.621(58) | 13.445(62) | 5.313(13) | 14.77(12) |
| | | 40 | 13.327(21) | 5.2872(52) | 14.552(40) | 13.384(40) | 5.3001(92) | 14.654(78) |
| | 22 | 28 | 13.533(30) | 5.3280(73) | 14.918(58) | 13.667(43) | 5.355(11) | 15.164(89) |
| | | 34 | 13.408(28) | 5.3040(75) | 14.675(56) | 13.485(94) | 5.309(20) | 14.88(18) |
| | | 40 | 13.458(21) | 5.3139(46) | 14.774(42) | 13.465(46) | 5.309(11) | 14.826(89) |
| 0.38683 | 28 | 38 | – | – | – | 24.156(50) | 9.449(12) | 26.834(99) |
| | | 42 | – | – | – | 24.191(50) | 9.461(11) | 26.830(99) |
| | | 46 | – | – | – | 24.096(43) | 9.451(10) | 26.610(84) |

Table 8: SU(5) finite-volume scale-setting results with TBCs and no improvement, with and without projection onto the $Q = 0$ topological sector. Empty cells correspond to simulation points for which we were not able to use the PTBC algorithm to sample $Q$ correctly.

| Primed, $N = 8$, Unimproved | | | | | | | | |
|---|---|---|---|---|---|---|---|---|
| | | | Any $Q$ | | | $Q = 0$ | | |
| $b$ | $L_s$ | $L$ | $t'_0/a^2$ | $t'_1/a^2$ | $w'^2_0/a^2$ | $t'_0/a^2$ | $t'_1/a^2$ | $w'^2_0/a^2$ |
| 0.35867 | 6 | 14 | 4.0604(58) | 1.5935(11) | 4.514(11) | 4.1283(46) | 1.60449(86) | 4.6615(95) |
| | | 16 | 4.0170(42) | 1.5857(10) | 4.4307(88) | 4.0764(35) | 1.59579(88) | 4.5536(82) |
| | | 18 | 4.0158(30) | 1.58539(60) | 4.4286(58) | 4.0671(41) | 1.59426(81) | 4.5328(82) |
| | 8 | 14 | 4.0688(34) | 1.60001(65) | 4.5048(67) | 4.1223(41) | 1.6086(18) | 4.6191(86) |
| | | 16 | 4.0587(28) | 1.59821(63) | 4.4857(54) | 4.0930(37) | 1.60394(79) | 4.5567(74) |
| | | 18 | 4.0600(18) | 1.59840(42) | 4.4877(37) | 4.0840(25) | 1.60236(63) | 4.5393(50) |
| | 10 | 14 | 4.0942(27) | 1.60485(54) | 4.5490(57) | 4.1255(55) | 1.6099(12) | 4.616(11) |
| | | 16 | 4.0844(30) | 1.60264(66) | 4.5314(61) | 4.1081(51) | 1.6072(11) | 4.578(10) |
| | | 18 | 4.0845(25) | 1.6027(12) | 4.5316(52) | 4.0984(42) | 1.60514(95) | 4.5624(83) |
| | 12 | 18 | 4.0928(27) | 1.60416(61) | 4.5483(53) | 4.1065(39) | 1.60628(94) | 4.5783(79) |
| 0.38352 | 12 | 28 | 15.384(99) | 5.924(21) | 17.31(20) | 15.56(12) | 5.955(24) | 17.68(26) |
| | | 32 | 15.345(45) | 5.9189(98) | 17.237(93) | 15.407(47) | 5.928(11) | 17.39(10) |
| | | 36 | 15.309(30) | 5.9192(67) | 17.112(62) | 15.470(43) | 5.9426(96) | 17.449(90) |
| | 16 | 28 | 15.446(50) | 5.959(11) | 17.33(10) | 15.514(60) | 5.970(13) | 17.46(12) |
| | | 32 | 15.460(41) | 5.959(10) | 17.362(86) | 15.518(51) | 5.968(10) | 17.49(11) |
| | | 36 | 15.449(30) | 5.9573(68) | 17.297(62) | 15.457(37) | 5.9566(79) | 17.327(75) |
| | 20 | 28 | 15.669(97) | 5.996(20) | 17.71(20) | 15.71(11) | 6.004(22) | 17.78(23) |
| | | 32 | 15.486(53) | 5.966(11) | 17.39(11) | 15.522(58) | 5.971(14) | 17.46(12) |
| | | 36 | 15.538(38) | 5.9720(81) | 17.453(76) | 15.533(38) | 5.9702(85) | 17.452(76) |
| | 24 | 36 | 15.531(39) | 5.9721(97) | 17.468(78) | 15.547(35) | 5.9742(91) | 17.501(71) |
| 0.40008 | 36 | 48 | – | – | – | 34.79(13) | 13.328(27) | 39.23(29) |
| | | 54 | – | – | – | 34.856(83) | 13.351(19) | 39.27(17) |
| | | 60 | – | – | – | 34.846(75) | 13.346(18) | 39.30(15) |

Table 9: SU(8) finite-volume scale-setting results with TBCs and no improvement, with and without projection onto the $Q = 0$ topological sector. Empty cells correspond to simulation points for which we were not able to use the PTBC algorithm to sample $Q$ correctly.

### 1.2.2 Improved

| Primed, $N=3$, Improved | | | | | | | | |
|---|---|---|---|---|---|---|---|---|
| | | | Any $Q$ | | | $Q=0$ | | |
| $b$ | $L_s$ | $L$ | $t'_0/a^2$ | $t'_1/a^2$ | $w'^2_0/a^2$ | $t'_0/a^2$ | $t'_1/a^2$ | $w'^2_0/a^2$ |
| 0.35883 | 16 | 24 | 12.631(44) | 5.277(11) | 13.253(76) | 13.710(67) | 5.482(16) | 15.41(15) |
| | | 30 | 12.261(43) | 5.202(12) | 12.614(72) | 12.783(66) | 5.309(16) | 13.52(12) |
| | | 36 | 12.167(21) | 5.1791(61) | 12.478(35) | 12.441(48) | 5.236(12) | 12.943(80) |
| | 20 | 24 | 12.521(36) | 5.2512(86) | 13.080(60) | 13.142(55) | 5.372(12) | 14.25(11) |
| | | 30 | 12.404(26) | 5.2300(64) | 12.852(43) | 12.718(42) | 5.291(10) | 13.408(72) |
| | | 36 | 12.407(24) | 5.2313(65) | 12.844(39) | 12.615(46) | 5.275(12) | 13.206(77) |
| | 24 | 24 | 12.548(21) | 5.2555(54) | 13.117(37) | 12.969(46) | 5.340(12) | 13.886(84) |
| | | 30 | 12.461(25) | 5.2394(59) | 12.949(42) | 12.720(43) | 5.294(11) | 13.388(76) |
| | | 36 | 12.447(24) | 5.2374(66) | 12.922(39) | 12.615(44) | 5.275(12) | 13.186(73) |
| 0.37583 | 18 | 38 | 26.48(34) | 11.36(11) | 27.07(54) | 28.84(60) | 11.79(16) | 31.6(1.2) |
| | | 46 | 26.59(18) | 11.368(57) | 27.28(30) | 27.48(25) | 11.550(68) | 28.83(43) |
| | | 54 | 26.01(16) | 11.238(45) | 26.37(24) | 26.83(22) | 11.395(59) | 27.79(36) |
| | 24 | 38 | 27.73(24) | 11.711(66) | 28.71(38) | 29.25(47) | 12.01(11) | 31.54(88) |
| | | 46 | 27.55(19) | 11.660(50) | 28.47(31) | 28.68(26) | 11.920(63) | 30.33(46) |
| | | 54 | 27.25(12) | 11.595(31) | 27.95(19) | 28.08(21) | 11.781(62) | 29.37(35) |
| | 30 | 38 | 28.46(16) | 11.881(42) | 29.88(28) | 29.29(27) | 12.036(67) | 31.42(51) |
| | | 46 | 28.32(19) | 11.836(51) | 29.54(32) | 28.63(22) | 11.894(60) | 30.08(38) |
| | | 54 | 27.68(22) | 11.664(63) | 28.64(37) | 28.22(41) | 11.765(99) | 29.55(70) |
| 0.38844 | 24 | 50 | 49.32(65) | 20.62(15) | 52.2(1.1) | 52.48(73) | 21.27(14) | 58.2(1.6) |
| | | 60 | 47.25(38) | 20.25(11) | 48.32(64) | 49.28(64) | 20.64(21) | 51.7(1.1) |
| | 32 | 50 | 51.1(2.2) | 21.05(72) | 54.8(3.8) | 52.7(3.1) | 21.41(84) | 57.7(5.0) |
| | | 60 | 49.50(35) | 20.95(11) | 51.09(58) | 50.23(58) | 21.12(16) | 52.4(1.0) |

Table 10: SU(3) finite-volume scale-setting results with TBCs and improvement of lattice artifacts, with and without projection onto the $Q=0$ topological sector.

| Primed, $N = 5$, Improved | | | | | | | | |
|---|---|---|---|---|---|---|---|---|
| | | | Any $Q$ | | | $Q = 0$ | | |
| $b$ | $L_s$ | $L$ | $t'_0/a^2$ | $t'_1/a^2$ | $w'^2_0/a^2$ | $t'_0/a^2$ | $t'_1/a^2$ | $w'^2_0/a^2$ |
| | | 18 | 6.0298(52) | 2.3579(11) | 6.643(10) | 6.1413(77) | 2.3774(16) | 6.871(16) |
| | 12 | 22 | 6.0100(71) | 2.3561(15) | 6.579(13) | 6.082(13) | 2.3694(27) | 6.725(25) |
| | | 26 | 6.0016(48) | 2.3539(11) | 6.5644(91) | 6.0490(99) | 2.3620(20) | 6.656(19) |
| | | 18 | 6.0570(76) | 2.3624(17) | 6.696(16) | 6.143(10) | 2.3781(26) | 6.867(25) |
| 0.35971 | 14 | 22 | 6.0426(69) | 2.3609(15) | 6.648(13) | 6.087(11) | 2.3695(27) | 6.733(21) |
| | | 26 | 6.0379(55) | 2.3598(13) | 6.632(10) | 6.0754(86) | 2.3661(19) | 6.707(17) |
| | | 18 | 6.0513(50) | 2.3604(11) | 6.6895(97) | 6.109(13) | 2.3700(26) | 6.814(25) |
| | 16 | 22 | 6.0281(57) | 2.3571(12) | 6.625(11) | 6.0825(77) | 2.3659(17) | 6.736(15) |
| | | 26 | 6.0414(47) | 2.3599(12) | 6.6442(90) | 6.064(12) | 2.3629(25) | 6.696(24) |
| | | 28 | 13.122(37) | 5.1903(94) | 14.320(68) | 13.466(49) | 5.248(12) | 15.02(10) |
| | 14 | 34 | 13.113(45) | 5.185(10) | 14.294(83) | 13.358(58) | 5.225(13) | 14.79(11) |
| | | 40 | 13.105(32) | 5.1788(90) | 14.312(59) | 13.242(45) | 5.203(10) | 14.581(85) |
| | | 28 | 13.370(45) | 5.2349(87) | 14.748(86) | 13.593(32) | 5.2741(75) | 15.206(65) |
| 0.37504 | 18 | 34 | 13.331(31) | 5.2338(70) | 14.619(58) | 13.393(62) | 5.243(12) | 14.77(12) |
| | | 40 | 13.278(21) | 5.2174(52) | 14.551(40) | 13.334(40) | 5.2301(92) | 14.653(78) |
| | | 28 | 13.481(30) | 5.2566(73) | 14.932(59) | 13.614(43) | 5.283(11) | 15.179(89) |
| | 22 | 34 | 13.358(28) | 5.2336(75) | 14.672(56) | 13.434(93) | 5.239(20) | 14.87(18) |
| | | 40 | 13.409(21) | 5.2436(46) | 14.772(42) | 13.416(46) | 5.239(11) | 14.824(89) |
| | | 38 | – | – | – | 24.103(50) | 9.378(11) | 26.846(99) |
| 0.38683 | 28 | 42 | – | – | – | 24.138(50) | 9.391(11) | 26.831(99) |
| | | 46 | – | – | – | 24.045(43) | 9.381(10) | 26.607(84) |

Table 11: SU(5) finite-volume scale-setting results with TBCs and improvement of lattice artifacts, with and without projection onto the $Q = 0$ topological sector. Empty cells correspond to simulation points for which we were not able to use the PTBC algorithm to sample $Q$ correctly.

| Primed, $N=8$, Improved | | | | | | | | |
|---|---|---|---|---|---|---|---|---|
| | | | Any $Q$ | | | $Q=0$ | | |
| $b$ | $L_s$ | $L$ | $t'_0/a^2$ | $t'_1/a^2$ | $w'^2_0/a^2$ | $t'_0/a^2$ | $t'_1/a^2$ | $w'^2_0/a^2$ |
| 0.35867 | 6 | 14 | 4.0093(58) | 1.5170(11) | 4.542(12) | 4.0769(45) | 1.52743(82) | 4.6932(97) |
| | | 16 | 3.9639(42) | 1.51052(98) | 4.4399(89) | 4.0226(35) | 1.52018(87) | 4.5651(84) |
| | | 18 | 3.9637(30) | 1.51066(58) | 4.4289(58) | 4.0145(41) | 1.51915(78) | 4.5339(83) |
| | 8 | 14 | 4.0179(34) | 1.52393(63) | 4.5339(69) | 4.0711(41) | 1.5321(17) | 4.6510(88) |
| | | 16 | 4.0053(28) | 1.52326(61) | 4.4965(55) | 4.0391(37) | 1.52873(77) | 4.5689(76) |
| | | 18 | 4.0075(18) | 1.52386(41) | 4.4888(37) | 4.0312(24) | 1.52765(61) | 4.5408(50) |
| | 10 | 14 | 4.0433(27) | 1.52872(53) | 4.5787(59) | 4.0744(55) | 1.5335(12) | 4.648(11) |
| | | 16 | 4.0307(30) | 1.52761(64) | 4.5425(62) | 4.0542(51) | 1.5320(11) | 4.591(11) |
| | | 18 | 4.0318(25) | 1.5281(12) | 4.5323(52) | 4.0455(42) | 1.53047(93) | 4.5635(84) |
| | 12 | 18 | 4.0402(27) | 1.52947(59) | 4.5489(54) | 4.0537(39) | 1.53149(91) | 4.5792(80) |
| 0.38352 | 12 | 28 | 15.333(99) | 5.850(21) | 17.33(20) | 15.51(12) | 5.881(24) | 17.71(27) |
| | | 32 | 15.291(44) | 5.8457(98) | 17.245(93) | 15.353(47) | 5.854(11) | 17.40(10) |
| | | 36 | 15.258(30) | 5.8464(67) | 17.111(62) | 15.418(43) | 5.8694(95) | 17.449(90) |
| | 16 | 28 | 15.395(50) | 5.885(10) | 17.36(10) | 15.462(60) | 5.896(13) | 17.49(12) |
| | | 32 | 15.406(41) | 5.8856(99) | 17.371(86) | 15.464(51) | 5.895(10) | 17.50(11) |
| | | 36 | 15.397(30) | 5.8847(67) | 17.298(62) | 15.405(37) | 5.8840(78) | 17.327(75) |
| | 20 | 28 | 15.617(97) | 5.922(19) | 17.74(20) | 15.66(11) | 5.930(22) | 17.81(24) |
| | | 32 | 15.432(53) | 5.893(11) | 17.40(11) | 15.468(58) | 5.898(13) | 17.46(12) |
| | | 36 | 15.485(38) | 5.8994(81) | 17.453(76) | 15.481(38) | 5.8975(84) | 17.452(77) |
| | 24 | 36 | 15.479(39) | 5.8995(97) | 17.468(78) | 15.495(35) | 5.9015(90) | 17.500(72) |
| 0.40008 | 36 | 48 | – | – | – | 34.74(13) | 13.256(27) | 39.24(29) |
| | | 54 | – | – | – | 34.804(83) | 13.279(19) | 39.27(17) |
| | | 60 | – | – | – | 34.795(75) | 13.274(18) | 39.30(15) |

Table 12: SU(8) finite-volume scale-setting results with TBCs and improvement of lattice artifacts, with and without projection onto the $Q=0$ topological sector. Empty cells correspond to simulation points for which we were not able to use the PTBC algorithm to sample $Q$ correctly.

# 2 Infinite-volume scales

## 2.1 $N$-by-$N$ fit strategy

### 2.1.1 With and without topological projection

| Unimproved — $N$-by-$N$ fit strategy | | | | | | | |
|---|---|---|---|---|---|---|---|
| | | Any $Q$ | | | $Q = 0$ | | |
| $N$ | $b$ | $t_0/a^2$ | $t_1/a^2$ | $w_0^2/a^2$ | $t_0/a^2$ | $t_1/a^2$ | $w_0^2/a^2$ |
| | 0.35883 | 12.550(35) | 5.3088(76) | 13.054(75) | 12.455(63) | 5.289(16) | 12.88(11) |
| 3 | 0.37583 | 28.02(14) | 11.795(34) | 29.19(25) | 27.96(19) | 11.801(51) | 28.99(34) |
| | 0.38844 | 50.95(36) | 21.26(10) | 53.59(64) | 49.30(58) | 20.93(17) | 50.71(96) |
| | 0.35971 | 6.648(11) | 2.7478(23) | 7.129(39) | 6.632(24) | 2.7403(46) | 7.132(86) |
| 5 | 0.37504 | 14.676(29) | 6.0114(60) | 15.835(88) | 14.583(56) | 5.982(11) | 15.75(18) |
| | 0.38683 | – | – | – | 26.10(11) | 10.652(22) | 28.29(37) |
| | 0.35867 | 4.6007(73) | 1.8881(10) | 4.985(23) | 4.613(21) | 1.8908(32) | 4.988(44) |
| 8 | 0.38352 | 17.521(33) | 7.0699(62) | 19.210(95) | 17.503(85) | 7.066(13) | 19.09(18) |
| | 0.40008 | – | – | – | 39.21(16) | 15.795(25) | 42.86(35) |

Table 13: Infinite-volume scale-setting results with TBCs and no improvement, with and without projection onto the $Q = 0$ topological sector. Data points at different values of $N$ were fitted independently (see Eq. (38) and Eq. (40) in the text). Empty cells correspond to simulation points for which we were not able to use the PTBC algorithm to sample $Q$ correctly.

| Improved — $N$-by-$N$ fit strategy | | | | | | | |
|---|---|---|---|---|---|---|---|
| | | Any $Q$ | | | $Q = 0$ | | |
| $N$ | $b$ | $t_0/a^2$ | $t_1/a^2$ | $w_0^2/a^2$ | $t_0/a^2$ | $t_1/a^2$ | $w_0^2/a^2$ |
| | 0.35883 | 12.506(36) | 5.2449(75) | 13.048(75) | 12.413(63) | 5.225(16) | 12.87(11) |
| 3 | 0.37583 | 27.98(14) | 11.733(34) | 29.18(25) | 27.93(20) | 11.737(51) | 28.98(34) |
| | 0.38844 | 50.93(36) | 21.20(10) | 53.58(64) | 49.28(58) | 20.87(17) | 50.69(96) |
| | 0.35971 | 6.600(12) | 2.6808(22) | 7.124(38) | 6.585(24) | 2.6737(45) | 7.128(86) |
| 5 | 0.37504 | 14.631(30) | 5.9457(60) | 15.829(87) | 14.539(56) | 5.916(11) | 15.74(18) |
| | 0.38683 | – | – | – | 26.07(11) | 10.586(22) | 28.27(37) |
| | 0.35867 | 4.5494(73) | 1.8190(10) | 4.986(22) | 4.561(21) | 1.8216(30) | 4.991(45) |
| 8 | 0.38352 | 17.473(34) | 7.0055(62) | 19.204(92) | 17.451(84) | 7.000(13) | 19.10(18) |
| | 0.40008 | – | – | – | 39.16(16) | 15.728(25) | 42.86(35) |

Table 14: Infinite-volume scale-setting results with TBCs and improvement of lattice artifacts, with and without projection onto the $Q = 0$ topological sector. Data points at different values of $N$ were fitted independently (see Eq. (38) and Eq. (40) in the text). Empty cells correspond to simulation points for which we were not able to use the PTBC algorithm to sample $Q$ correctly.

| Primed, Unimproved — $N$-by-$N$ fit strategy | | | | | | | |
|---|---|---|---|---|---|---|---|
| | | Any $Q$ | | | $Q=0$ | | |
| $N$ | $b$ | $t'_0/a^2$ | $t'_1/a^2$ | $w'^2_0/a^2$ | $t'_0/a^2$ | $t'_1/a^2$ | $w'^2_0/a^2$ |
| | 0.35883 | 12.550(35) | 5.3088(76) | 13.054(75) | 12.455(63) | 5.289(16) | 12.88(11) |
| 3 | 0.37583 | 28.02(14) | 11.795(34) | 29.19(25) | 27.96(19) | 11.801(51) | 28.99(34) |
| | 0.38844 | 50.95(36) | 21.26(10) | 53.59(64) | 49.30(58) | 20.93(17) | 50.71(96) |
| | 0.35971 | 6.1069(96) | 2.4334(18) | 6.696(32) | 6.091(20) | 2.4270(37) | 6.697(73) |
| 5 | 0.37504 | 13.474(25) | 5.3133(48) | 14.871(74) | 13.388(48) | 5.2890(93) | 14.79(16) |
| | 0.38683 | – | – | – | 23.957(94) | 9.408(18) | 26.56(31) |
| | 0.35867 | 4.1034(56) | 1.60477(79) | 4.585(21) | 4.114(16) | 1.6067(26) | 4.582(36) |
| 8 | 0.38352 | 15.602(27) | 5.9789(47) | 17.657(85) | 15.589(65) | 5.976(10) | 17.53(15) |
| | 0.40008 | – | – | – | 34.91(12) | 13.348(20) | 39.37(28) |

Table 15: Infinite-volume scale-setting results with TBCs and no improvement, with and without projection onto the $Q = 0$ topological sector. Data points at different values of $N$ were fitted independently (see Eq. (38) and Eq. (40) in the text). Empty cells correspond to simulation points for which we were not able to use the PTBC algorithm to sample $Q$ correctly.

| Primed, Improved — $N$-by-$N$ fit strategy | | | | | | | |
|---|---|---|---|---|---|---|---|
| | | Any $Q$ | | | $Q=0$ | | |
| $N$ | $b$ | $t'_0/a^2$ | $t'_1/a^2$ | $w'^2_0/a^2$ | $t'_0/a^2$ | $t'_1/a^2$ | $w'^2_0/a^2$ |
| | 0.35883 | 12.506(36) | 5.2449(75) | 13.048(75) | 12.413(63) | 5.225(16) | 12.87(11) |
| 3 | 0.37583 | 27.98(14) | 11.733(34) | 29.18(25) | 27.93(20) | 11.737(51) | 28.98(34) |
| | 0.38844 | 50.93(36) | 21.20(10) | 53.58(64) | 49.28(58) | 20.87(17) | 50.69(96) |
| | 0.35971 | 6.0585(99) | 2.3623(18) | 6.693(32) | 6.044(20) | 2.3561(36) | 6.695(73) |
| 5 | 0.37504 | 13.428(26) | 5.2434(48) | 14.868(74) | 13.344(47) | 5.2188(93) | 14.78(16) |
| | 0.38683 | – | – | – | 23.919(95) | 9.337(18) | 26.55(32) |
| | 0.35867 | 4.0509(57) | 1.52996(75) | 4.584(20) | 4.061(16) | 1.5318(23) | 4.583(37) |
| 8 | 0.38352 | 15.554(27) | 5.9086(46) | 17.651(83) | 15.536(65) | 5.904(11) | 17.54(15) |
| | 0.40008 | – | – | – | 34.86(12) | 13.276(20) | 39.37(28) |

Table 16: Infinite-volume scale-setting results with TBCs and improvement of lattice artifacts, with and without projection onto the $Q = 0$ topological sector. Data points at different values of $N$ were fitted independently (see Eq. (38) and Eq. (40) in the text). Empty cells correspond to simulation points for which we were not able to use the PTBC algorithm to sample $Q$ correctly.

| Unimproved — $N$-by-$N$ fit strategy | | | | | | | | | | | | |
|---|---|---|---|---|---|---|---|---|---|---|---|---|
| | | Any $Q$ | | | | | $Q = 0$ | | | | | |
| Scale | $N$ | $N^2\hat{A}$ | $M$ | d.o.f. | $\chi^2_{\text{red}}$ | $p$-value | $N^2\hat{A}$ | $M$ | $N^2\hat{C}$ | d.o.f. | $\chi^2_{\text{red}}$ | $p$-value |
| | 3 | 13.2(5.5) | 2.52(33) | 3 | 0.50 | 68% | 29(10) | 2.75(30) | 13.6(2.7) | 8 | 0.47 | 88% |
| $t_0/a^2$ | 5 | 21(16) | 2.69(57) | 2 | 2.85 | 6% | 16(14) | 2.38(70) | 12.1(3.5) | 8 | 0.38 | 93% |
| | 8 | 11.1(3.0) | 2.06(32) | 4 | 0.61 | 65% | 5.5(5.9) | 1.50(69) | 4.2(7.5) | 8 | 0.50 | 86% |
| | 3 | 13.2(5.5) | 2.52(33) | 3 | 0.50 | 68% | 29(10) | 2.75(30) | 13.6(2.7) | 8 | 0.47 | 88% |
| $t'_0/a^2$ | 5 | 23(17) | 2.68(56) | 2 | 2.88 | 6% | 17(16) | 2.39(69) | 13.4(4.0) | 8 | 0.36 | 94% |
| | 8 | 11.7(3.2) | 2.05(30) | 4 | 0.56 | 69% | 4.9(5.8) | 1.50(71) | 3.0(8.9) | 8 | 0.46 | 88% |
| | 3 | 17.9(9.2) | 2.08(27) | 3 | 0.31 | 82% | 30(13) | 2.11(26) | 36.5(8.7) | 8 | 0.58 | 79% |
| $t_1/a^2$ | 5 | 28(28) | 2.18(48) | 2 | 2.55 | 8% | 31(36) | 2.21(59) | 37(12) | 8 | 0.25 | 98% |
| | 8 | 20.2(6.7) | 2.04(23) | 4 | 0.19 | 94% | 9.3(6.7) | 1.81(58) | 1(29) | 8 | 0.31 | 96% |
| | 3 | 17.9(9.2) | 2.08(27) | 3 | 0.31 | 82% | 30(13) | 2.11(26) | 36.5(8.7) | 8 | 0.58 | 79% |
| $t'_1/a^2$ | 5 | 27(29) | 2.08(47) | 2 | 2.46 | 9% | 31(38) | 2.13(58) | 43(14) | 8 | 0.24 | 98% |
| | 8 | 21.4(7.5) | 1.99(22) | 4 | 0.17 | 95% | 10.8(7.7) | 1.83(65) | 1(36) | 8 | 0.30 | 97% |
| | 3 | 10.7(4.8) | 2.13(36) | 3 | 0.54 | 66% | 33(12) | 2.56(32) | 20.9(4.3) | 8 | 0.38 | 93% |
| $w_0^2/a^2$ | 5 | 11.8(9.1) | 1.97(65) | 2 | 1.97 | 14% | 9.9(8.8) | 1.63(76) | 17.8(5.4) | 8 | 0.41 | 92% |
| | 8 | 10.2(2.7) | 1.57(38) | 4 | 0.48 | 75% | 13(10) | 1.50(53) | 17(12) | 8 | 0.52 | 84% |
| | 3 | 10.7(4.8) | 2.13(36) | 3 | 0.54 | 66% | 33(12) | 2.56(32) | 20.9(4.3) | 8 | 0.38 | 93% |
| $w_0'^2/a^2$ | 5 | 13(10) | 2.02(63) | 2 | 1.98 | 14% | 10.2(9.3) | 1.65(74) | 19.1(5.9) | 8 | 0.40 | 92% |
| | 8 | 9.6(2.6) | 1.50(37) | 4 | 0.55 | 70% | 13(10) | 1.50(49) | 19(13) | 8 | 0.61 | 77% |

Table 17: Best-fit parameters and quality of the volume dependence of the scales with TBCs and no improvement, with and without projection onto the $Q = 0$ topological sector. Data points at different values of $N$ were fitted independently (see Eq. (38) and Eq. (40) in the text).

| Improved — $N$-by-$N$ fit strategy | | | | | | | | | | | | |
|---|---|---|---|---|---|---|---|---|---|---|---|---|
| | | Any $Q$ | | | | | $Q = 0$ | | | | | |
| Scale | $N$ | $N^2\hat{A}$ | $M$ | d.o.f. | $\chi^2_{\text{red}}$ | $p$-value | $N^2\hat{A}$ | $M$ | $N^2\hat{C}$ | d.o.f. | $\chi^2_{\text{red}}$ | $p$-value |
| | 3 | 12.7(5.3) | 2.49(32) | 3 | 0.50 | 68% | 29(10) | 2.73(30) | 13.5(2.7) | 8 | 0.47 | 88% |
| $t_0/a^2$ | 5 | 19(14) | 2.63(56) | 2 | 2.78 | 6% | 15(14) | 2.38(72) | 11.5(3.6) | 8 | 0.39 | 93% |
| | 8 | 11.0(3.0) | 2.03(32) | 4 | 0.63 | 64% | 5.6(5.8) | 1.50(67) | 4.4(7.5) | 8 | 0.51 | 85% |
| | 3 | 12.7(5.3) | 2.49(32) | 3 | 0.50 | 68% | 29(10) | 2.73(30) | 13.5(2.7) | 8 | 0.47 | 88% |
| $t'_0/a^2$ | 5 | 21(16) | 2.61(54) | 2 | 2.80 | 6% | 17(16) | 2.39(71) | 12.7(4.1) | 8 | 0.38 | 93% |
| | 8 | 11.5(3.2) | 2.02(30) | 4 | 0.59 | 67% | 5.0(5.8) | 1.50(69) | 3.2(8.9) | 8 | 0.48 | 87% |
| | 3 | 17.7(9.0) | 2.06(26) | 3 | 0.33 | 80% | 30(13) | 2.10(26) | 37.0(8.9) | 8 | 0.58 | 80% |
| $t_1/a^2$ | 5 | 27(27) | 2.15(46) | 2 | 2.47 | 8% | 34(41) | 2.25(60) | 37(13) | 8 | 0.27 | 98% |
| | 8 | 21.3(6.9) | 2.01(22) | 4 | 0.45 | 77% | 10.2(7.0) | 1.81(55) | 1(29) | 8 | 0.35 | 95% |
| | 3 | 17.7(9.0) | 2.06(26) | 3 | 0.33 | 80% | 30(13) | 2.10(26) | 37.0(8.9) | 8 | 0.58 | 80% |
| $t'_1/a^2$ | 5 | 27(28) | 2.05(46) | 2 | 2.36 | 9% | 36(44) | 2.18(59) | 44(15) | 8 | 0.26 | 98% |
| | 8 | 24.4(8.5) | 1.99(22) | 4 | 0.52 | 72% | 13.4(9.5) | 1.88(64) | 1(37) | 8 | 0.35 | 95% |
| | 3 | 10.7(4.8) | 2.13(36) | 3 | 0.50 | 68% | 33(12) | 2.56(32) | 21.0(4.3) | 8 | 0.38 | 93% |
| $w_0^2/a^2$ | 5 | 11.8(9.2) | 1.98(65) | 2 | 1.93 | 15% | 10.1(8.8) | 1.63(74) | 18.6(5.4) | 8 | 0.39 | 92% |
| | 8 | 10.6(2.9) | 1.62(38) | 4 | 0.47 | 76% | 13(10) | 1.50(53) | 17(12) | 8 | 0.49 | 87% |
| | 3 | 10.7(4.8) | 2.13(36) | 3 | 0.50 | 68% | 33(12) | 2.56(32) | 21.0(4.3) | 8 | 0.38 | 93% |
| $w_0'^2/a^2$ | 5 | 13(10) | 2.02(64) | 2 | 1.93 | 14% | 10.2(9.3) | 1.64(74) | 19.5(5.9) | 8 | 0.39 | 93% |
| | 8 | 9.8(2.7) | 1.53(37) | 4 | 0.52 | 72% | 13(10) | 1.50(49) | 20(13) | 8 | 0.57 | 80% |

Table 18: Best-fit parameters and quality of the volume dependence of the scales with TBCs and improvement of lattice artifacts, with and without projection onto the $Q = 0$ topological sector. Data points at different values of $N$ were fitted independently (see Eq. (38) and Eq. (40) in the text).

### 2.1.2 Combined final results

| | | Unimproved — $N$-by-$N$ fit strategy | | | | | |
|---|---|---|---|---|---|---|---|
| $N$ | $b$ | $t_0/a^2$ | $t_1/a^2$ | $w_0^2/a^2$ | $t'_0/a^2$ | $t'_1/a^2$ | $w_0'^2/a^2$ |
| | 0.35883 | 12.528(35)[23] | 5.3052(76)[43] | 13.000(75)[44] | 12.528(35)[23] | 5.3052(76)[43] | 13.000(75)[44] |
| 3 | 0.37583 | 28.00(14)[1] | 11.797(34)[1] | 29.12(25)[2] | 28.00(14)[1] | 11.797(34)[1] | 29.12(25)[2] |
| | 0.38844 | 50.49(36)[63] | 21.17(10)[10] | 52.7(6)[1.1] | 50.49(36)[63] | 21.17(10)[10] | 52.7(6)[1.1] |
| | 0.35971 | 6.645(11)[2] | 2.7463(23)[20] | 7.129(39)[1] | 6.1041(96)[21] | 2.4322(18)[18] | 6.696(32)[1] |
| 5 | 0.37504 | 14.656(29)[25] | 6.005(6)[11] | 15.819(88)[7] | 13.455(25)[24] | 5.3081(48)[92] | 14.855(74)[8] |
| | 0.38683 | 26.10(11)[8] | 10.652(22)[17] | 28.29(37)[16] | 23.957(94)[71] | 9.408(18)[14] | 26.56(31)[14] |
| | 0.35867 | 4.6020(73)[13] | 1.8883(10)[4] | 4.986(23)[1] | 4.1045(56)[12] | 1.60494(79)[28] | 4.584(21)[1] |
| 8 | 0.38352 | 17.518(33)[1] | 7.0691(62)[2] | 19.184(95)[13] | 15.601(27)[1] | 5.9784(47)[2] | 17.626(85)[17] |
| | 0.40008 | 39.21(16)[1] | 15.795(25)[1] | 42.86(35)[7] | 34.91(12)[1] | 13.348(20)[1] | 39.37(28)[6] |

Table 19: Infinite-volume scale-setting results with TBCs and no improvement. Results with and without projection onto the $Q = 0$ topological sector are combined into a single value with a systematic error (shown between square brackets). Data points at different values of $N$ were fitted independently (see Eq. (38) and Eq. (40) in the text).

| | | Improved — $N$-by-$N$ fit strategy | | | | | |
|---|---|---|---|---|---|---|---|
| $N$ | $b$ | $t_0/a^2$ | $t_1/a^2$ | $w_0^2/a^2$ | $t'_0/a^2$ | $t'_1/a^2$ | $w_0'^2/a^2$ |
| | 0.35883 | 12.483(36)[22] | 5.2414(75)[41] | 12.993(75)[44] | 12.483(36)[22] | 5.2414(75)[41] | 12.993(75)[44] |
| 3 | 0.37583 | 27.96(14)[1] | 11.734(34)[1] | 29.11(25)[2] | 27.96(14)[1] | 11.734(34)[1] | 29.11(25)[2] |
| | 0.38844 | 50.47(36)[63] | 21.11(10)[10] | 52.7(6)[1.1] | 50.47(36)[63] | 21.11(10)[10] | 52.7(6)[1.1] |
| | 0.35971 | 6.597(12)[2] | 2.6794(22)[19] | 7.125(38)[1] | 6.0557(99)[18] | 2.3611(18)[17] | 6.693(32)[1] |
| 5 | 0.37504 | 14.611(30)[24] | 5.939(6)[11] | 15.813(87)[7] | 13.409(26)[24] | 5.2382(48)[94] | 14.852(74)[8] |
| | 0.38683 | 26.07(11)[8] | 10.586(22)[17] | 28.27(37)[16] | 23.919(95)[67] | 9.337(18)[14] | 26.55(32)[14] |
| | 0.35867 | 4.5507(73)[13] | 1.8193(10)[4] | 4.987(22)[1] | 4.0520(57)[11] | 1.53014(75)[28] | 4.584(20)[1] |
| 8 | 0.38352 | 17.470(34)[1] | 7.0045(62)[4] | 19.182(92)[11] | 15.552(27)[1] | 5.9079(46)[3] | 17.623(83)[16] |
| | 0.40008 | 39.16(16)[1] | 15.728(25)[1] | 42.86(35)[7] | 34.86(12)[1] | 13.276(20)[1] | 39.37(28)[6] |

Table 20: Infinite-volume scale-setting results with TBCs and improvement of lattice artifacts. Results with and without projection onto the $Q = 0$ topological sector are combined into a single value with a systematic error (shown between square brackets). Data points at different values of $N$ were fitted independently (see Eq. (38) and Eq. (40) in the text).

## 2.2 Global fit strategy

### 2.2.1 With and without topological projection

| Unimproved — Global fit strategy | | | | | | | |
|---|---|---|---|---|---|---|---|
| | | Any $Q$ | | | $Q=0$ | | |
| $N$ | $b$ | $t_0/a^2$ | $t_1/a^2$ | $w_0^2/a^2$ | $t_0/a^2$ | $t_1/a^2$ | $w_0^2/a^2$ |
| 3 | 0.35883 | 12.567(26) | 5.3105(56) | 13.091(57) | 12.534(53) | 5.298(13) | 13.02(10) |
| | 0.37583 | 28.05(13) | 11.800(32) | 29.25(23) | 28.12(18) | 11.818(46) | 29.26(32) |
| | 0.38844 | 50.99(35) | 21.27(10) | 53.66(62) | 49.66(55) | 20.98(16) | 51.28(90) |
| 5 | 0.35971 | 6.6545(74) | 2.7480(14) | 7.134(19) | 6.639(12) | 2.7434(26) | 7.104(26) |
| | 0.37504 | 14.688(24) | 6.0110(49) | 15.850(54) | 14.618(36) | 5.9922(80) | 15.730(75) |
| | 0.38683 | – | – | – | 26.129(61) | 10.664(14) | 28.16(13) |
| 8 | 0.35867 | 4.5953(36) | 1.88819(75) | 4.9680(92) | 4.5822(54) | 1.8851(12) | 4.945(12) |
| | 0.38352 | 17.501(24) | 7.0704(56) | 19.145(52) | 17.386(27) | 7.0439(63) | 18.934(56) |
| | 0.40008 | – | – | – | 39.021(66) | 15.764(16) | 42.59(14) |

Table 21: Infinite-volume scale-setting results with TBCs and no improvement, with and without projection onto the $Q = 0$ topological sector. Data points at all the values of $N$ were fitted together (see Eq. (44) and Eq. (45) in the text). Empty cells correspond to simulation points for which we were not able to use the PTBC algorithm to sample $Q$ correctly.

| Improved — Global fit strategy | | | | | | | |
|---|---|---|---|---|---|---|---|
| | | Any $Q$ | | | $Q=0$ | | |
| $N$ | $b$ | $t_0/a^2$ | $t_1/a^2$ | $w_0^2/a^2$ | $t_0/a^2$ | $t_1/a^2$ | $w_0^2/a^2$ |
| 3 | 0.35883 | 12.522(27) | 5.2462(55) | 13.079(56) | 12.494(53) | 5.234(13) | 13.00(10) |
| | 0.37583 | 28.01(13) | 11.737(32) | 29.23(23) | 28.09(18) | 11.754(46) | 29.22(32) |
| | 0.38844 | 50.97(35) | 21.21(10) | 53.63(62) | 49.66(55) | 20.91(16) | 51.20(90) |
| 5 | 0.35971 | 6.6067(75) | 2.6811(13) | 7.129(19) | 6.591(12) | 2.6768(25) | 7.099(26) |
| | 0.37504 | 14.643(24) | 5.9457(48) | 15.843(54) | 14.572(36) | 5.9268(80) | 15.722(75) |
| | 0.38683 | – | – | – | 26.086(62) | 10.598(14) | 28.15(13) |
| 8 | 0.35867 | 4.5441(36) | 1.81906(73) | 4.9696(91) | 4.5316(53) | 1.8163(11) | 4.947(12) |
| | 0.38352 | 17.454(24) | 7.0056(56) | 19.144(52) | 17.337(27) | 6.9779(63) | 18.933(56) |
| | 0.40008 | – | – | – | 38.975(66) | 15.698(16) | 42.58(14) |

Table 22: Infinite-volume scale-setting results with TBCs and improvement of lattice artifacts, with and without projection onto the $Q = 0$ topological sector. Data points at all the values of $N$ were fitted together (see Eq. (44) and Eq. (45) in the text). Empty cells correspond to simulation points for which we were not able to use the PTBC algorithm to sample $Q$ correctly.

| | | Primed, Unimproved — Global fit strategy | | | | | |
|---|---|---|---|---|---|---|---|
| | | Any $Q$ | | | $Q=0$ | | |
| $N$ | $b$ | $t'_0/a^2$ | $t'_1/a^2$ | $w'^2_0/a^2$ | $t'_0/a^2$ | $t'_1/a^2$ | $w'^2_0/a^2$ |
| 3 | 0.35883 | 12.571(26) | 5.3119(57) | 13.104(59) | 12.525(54) | 5.294(14) | 13.02(10) |
| | 0.37583 | 28.06(13) | 11.803(33) | 29.28(23) | 28.10(18) | 11.809(47) | 29.26(32) |
| | 0.38844 | 51.00(35) | 21.27(10) | 53.70(62) | 49.60(55) | 20.95(16) | 51.24(91) |
| 5 | 0.35971 | 6.1125(63) | 2.4333(11) | 6.704(18) | 6.0995(99) | 2.4300(20) | 6.677(23) |
| | 0.37504 | 13.483(20) | 5.3123(39) | 14.890(50) | 13.420(31) | 5.2976(64) | 14.776(68) |
| | 0.38683 | – | – | – | 23.990(52) | 9.420(11) | 26.47(11) |
| 8 | 0.35867 | 4.0996(30) | 1.60489(58) | 4.5684(80) | 4.0893(43) | 1.60283(86) | 4.5484(99) |
| | 0.38352 | 15.589(20) | 5.9793(42) | 17.596(46) | 15.495(22) | 5.9610(46) | 17.413(48) |
| | 0.40008 | – | – | – | 34.768(54) | 13.328(12) | 39.17(12) |

Table 23: Infinite-volume scale-setting results with TBCs and no improvement, with and without projection onto the $Q = 0$ topological sector. Data points at all the values of $N$ were fitted together (see Eq. (44) and Eq. (45) in the text). Empty cells correspond to simulation points for which we were not able to use the PTBC algorithm to sample $Q$ correctly.

| | | Primed, Improved — Global fit strategy | | | | | |
|---|---|---|---|---|---|---|---|
| | | Any $Q$ | | | $Q=0$ | | |
| $N$ | $b$ | $t'_0/a^2$ | $t'_1/a^2$ | $w'^2_0/a^2$ | $t'_0/a^2$ | $t'_1/a^2$ | $w'^2_0/a^2$ |
| 3 | 0.35883 | 12.528(27) | 5.2471(56) | 13.093(58) | 12.485(54) | 5.229(13) | 13.01(10) |
| | 0.37583 | 28.02(13) | 11.739(32) | 29.26(23) | 28.07(18) | 11.743(47) | 29.23(32) |
| | 0.38844 | 50.98(35) | 21.21(10) | 53.68(62) | 49.60(55) | 20.88(16) | 51.19(90) |
| 5 | 0.35971 | 6.0638(64) | 2.3622(10) | 6.701(17) | 6.0507(98) | 2.3591(19) | 6.674(23) |
| | 0.37504 | 13.437(20) | 5.2426(38) | 14.885(49) | 13.373(31) | 5.2281(63) | 14.769(67) |
| | 0.38683 | – | – | – | 23.946(52) | 9.350(11) | 26.46(11) |
| 8 | 0.35867 | 4.0470(30) | 1.53004(56) | 4.5686(80) | 4.0373(42) | 1.52830(80) | 4.5486(99) |
| | 0.38352 | 15.540(20) | 5.9089(42) | 17.593(45) | 15.445(22) | 5.8895(46) | 17.411(48) |
| | 0.40008 | – | – | – | 34.720(54) | 13.255(12) | 39.16(12) |

Table 24: Infinite-volume scale-setting results with TBCs and improvement of lattice artifacts, with and without projection onto the $Q = 0$ topological sector. Data points at all the values of $N$ were fitted together (see Eq. (44) and Eq. (45) in the text). Empty cells correspond to simulation points for which we were not able to use the PTBC algorithm to sample $Q$ correctly.

| | Unimproved — Global fit strategy | | | | | | | | | | |
|---|---|---|---|---|---|---|---|---|---|---|---|
| | Any $Q$ | | | | | $Q=0$ | | | | | |
| Scale | $M$ | $A_0$ | $A_1$ | $\chi^2_{\text{red}}$ | $p$-value | $M$ | $A_0$ | $A_1$ | $C$ | $\chi^2_{\text{red}}$ | $p$-value |
| $t_0/a^2$ | 2.34(19) | 15.1(2.5) | 3.9(1.8) | 0.93 | 51% | 2.42(19) | 19.1(3.8) | 0.5(1.1) | 11.7(2.0) | 0.80 | 77% |
| $t'_0/a^2$ | 2.31(18) | 16.0(2.8) | 5.4(1.9) | 0.94 | 51% | 2.41(19) | 19.2(4.0) | 0.4(1.0) | 12.3(2.1) | 0.76 | 82% |
| $t_1/a^2$ | 2.02(14) | 20.4(4.0) | 2.4(1.6) | 0.61 | 84% | 2.06(16) | 24.0(5.2) | -0.5(1.1) | 32.6(6.7) | 0.56 | 97% |
| $t'_1/a^2$ | 1.96(14) | 22.2(4.7) | 4.8(1.9) | 0.61 | 83% | 2.02(16) | 25.1(6.0) | 0.1(1.0) | 35.2(7.1) | 0.52 | 98% |
| $w^2_0/a^2$ | 1.93(22) | 14.5(2.4) | 6.5(2.6) | 0.73 | 73% | 2.13(21) | 21.8(5.0) | 1.8(1.5) | 18.5(3.1) | 0.69 | 89% |
| $w'^2_0/a^2$ | 1.87(21) | 14.2(2.5) | 7.2(2.6) | 0.79 | 66% | 2.09(21) | 20.2(4.8) | 1.3(1.4) | 19.1(3.2) | 0.71 | 88% |

Table 25: Best-fit parameters and quality of the volume dependence of the scales with TBCs and no improvement, with and without projection onto the $Q = 0$ topological sector. Data points at all the values of $N$ were fitted together (see Eq. (44) and Eq. (45) in the text). Fits with and without topological projection have 12 and 29 degrees of freedom respectively.

| Improved — Global fit strategy | | | | | | | | | | | |
|---|---|---|---|---|---|---|---|---|---|---|---|
| | Any $Q$ | | | | | $Q = 0$ | | | | | |
| Scale | $M$ | $A_0$ | $A_1$ | $\chi^2_{\text{red}}$ | $p$-value | $M$ | $A_0$ | $A_1$ | $C$ | $\chi^2_{\text{red}}$ | $p$-value |
| $t_0/a^2$ | 2.31(18) | 14.9(2.4) | 4.1(1.8) | 0.92 | 53% | 2.41(19) | 18.7(3.8) | 0.5(1.1) | 11.5(2.0) | 0.80 | 76% |
| $t'_0/a^2$ | 2.27(18) | 15.9(2.7) | 5.7(1.9) | 0.93 | 52% | 2.40(19) | 18.7(3.9) | 0.4(1.0) | 12.0(2.1) | 0.77 | 81% |
| $t_1/a^2$ | 2.01(14) | 22.6(4.4) | 3.4(1.8) | 0.67 | 79% | 2.07(17) | 26.0(5.8) | -0.2(1.1) | 32.7(6.9) | 0.59 | 96% |
| $t'_1/a^2$ | 1.98(13) | 26.3(5.6) | 6.5(2.1) | 0.68 | 77% | 2.06(17) | 29.1(7.3) | 0.7(1.1) | 35.6(7.4) | 0.53 | 98% |
| $w_0^2/a^2$ | 1.95(22) | 14.9(2.5) | 6.5(2.6) | 0.70 | 76% | 2.15(21) | 22.4(5.1) | 1.8(1.5) | 18.9(3.1) | 0.67 | 91% |
| $w_0'^2/a^2$ | 1.89(21) | 14.5(2.6) | 7.1(2.6) | 0.74 | 71% | 2.11(21) | 20.5(4.9) | 1.2(1.3) | 19.4(3.2) | 0.69 | 90% |

Table 26: Best-fit parameters and quality of the volume dependence of the scales with TBCs and improvement of lattice artifacts, with and without projection onto the $Q = 0$ topological sector. Data points at all the values of $N$ were fitted together (see Eq. (44) and Eq. (45) in the text). Fits with and without topological projection have 12 and 29 degrees of freedom respectively.

### 2.2.2 Combined final results

| Unimproved — Global fit strategy | | | | | | | |
|---|---|---|---|---|---|---|---|
| $N$ | $b$ | $t_0/a^2$ | $t_1/a^2$ | $w_0^2/a^2$ | $t_0'/a^2$ | $t_1'/a^2$ | $w_0'^2/a^2$ |
| 3 | 0.35883 | 12.561(26)[4] | 5.3085(56)[22] | 13.074(57)[8] | 12.562(26)[7] | 5.3092(57)[43] | 13.084(59)[11] |
| | 0.37583 | 28.07(13)[1] | 11.806(32)[1] | 29.25(23)[1] | 28.07(13)[1] | 11.805(33)[1] | 29.27(23)[1] |
| | 0.38844 | 50.60(35)[46] | 21.18(10)[8] | 52.90(62)[86] | 50.59(35)[50] | 21.18(10)[10] | 52.92(62)[91] |
| 5 | 0.35971 | 6.6501(74)[34] | 2.7470(14)[13] | 7.123(19)[5] | 6.1087(63)[27] | 2.4326(11)[9] | 6.694(18)[5] |
| | 0.37504 | 14.667(24)[21] | 6.0060(49)[65] | 15.809(54)[29] | 13.464(20)[19] | 5.3083(39)[50] | 14.850(50)[29] |
| | 0.38683 | 26.129(61)[81] | 10.664(14)[15] | 28.16(13)[16] | 23.990(52)[66] | 9.420(11)[11] | 26.47(11)[14] |
| 8 | 0.35867 | 4.5912(36)[45] | 1.8873(7)[11] | 4.9593(92)[64] | 4.0962(30)[35] | 1.60425(58)[70] | 4.5604(80)[57] |
| | 0.38352 | 17.450(24)[52] | 7.059(6)[12] | 19.047(52)[88] | 15.546(20)[41] | 5.9709(42)[79] | 17.509(46)[76] |
| | 0.40008 | 39.021(66)[37] | 15.764(16)[7] | 42.59(14)[8] | 34.768(54)[28] | 13.328(12)[4] | 39.17(12)[6] |

Table 27: Infinite-volume scale-setting results with TBCs and no improvement. Results with and without projection onto the $Q = 0$ topological sector are combined into a single value with a systematic error (shown between square brackets). Data points at all the values of $N$ were fitted together (see Eq. (44) and Eq. (45) in the text).

| Improved — Global fit strategy | | | | | | | |
|---|---|---|---|---|---|---|---|
| $N$ | $b$ | $t_0/a^2$ | $t_1/a^2$ | $w_0^2/a^2$ | $t_0'/a^2$ | $t_1'/a^2$ | $w_0'^2/a^2$ |
| 3 | 0.35883 | 12.517(27)[3] | 5.2443(55)[21] | 13.061(56)[10] | 12.519(27)[6] | 5.2445(56)[42] | 13.072(58)[12] |
| | 0.37583 | 28.04(13)[1] | 11.743(32)[1] | 29.23(23)[1] | 28.04(13)[1] | 11.741(32)[1] | 29.25(23)[1] |
| | 0.38844 | 50.58(35)[44] | 21.12(10)[8] | 52.85(62)[90] | 50.58(35)[49] | 21.12(10)[10] | 52.88(62)[93] |
| 5 | 0.35971 | 6.6021(75)[35] | 2.6801(13)[12] | 7.119(19)[5] | 6.0599(64)[28] | 2.3615(10)[8] | 6.691(17)[5] |
| | 0.37504 | 14.622(24)[21] | 5.9406(48)[65] | 15.802(54)[30] | 13.418(20)[20] | 5.2387(38)[49] | 14.845(49)[30] |
| | 0.38683 | 26.086(62)[79] | 10.598(14)[15] | 28.15(13)[16] | 23.946(52)[64] | 9.350(11)[11] | 26.46(11)[14] |
| 8 | 0.35867 | 4.5401(36)[41] | 1.81826(73)[96] | 4.9610(91)[65] | 4.0437(30)[32] | 1.52947(56)[55] | 4.5607(80)[57] |
| | 0.38352 | 17.401(24)[52] | 6.993(6)[12] | 19.046(52)[88] | 15.496(20)[42] | 5.9000(42)[85] | 17.507(45)[75] |
| | 0.40008 | 38.975(66)[36] | 15.698(16)[7] | 42.58(14)[8] | 34.720(54)[27] | 13.255(12)[4] | 39.16(12)[6] |

Table 28: Infinite-volume scale-setting results with TBCs and improvement of lattice artifacts. Results with and without projection onto the $Q = 0$ topological sector are combined into a single value with a systematic error (shown between square brackets). Data points at all the values of $N$ were fitted together (see Eq. (44) and Eq. (45) in the text).

# 3 Continuum scale ratios

## 3.1 $N$-by-$N$ fit strategy

| $N$-by-$N$ fit strategy | | | | | | | | | | | |
|---|---|---|---|---|---|---|---|---|---|---|---|
| | | Unimproved | | | | | Improved | | | | |
| Ratio | $N$ | R | $C$ | $D$ | $\chi^2_{\text{red}}$ | $p$-value | R | $C$ | $D$ | $\chi^2_{\text{red}}$ | $p$-value |
| $t_1/t_0$ | 3 | 0.4188(33) | – | 1.13(93) | 0.07 | 79% | 0.4187(33) | – | 0.29(92) | 0.07 | 79% |
| | 5 | 0.4066(15) | – | 0.88(26) | 0.03 | 86% | 0.4066(15) | – | -0.05(25) | 0.05 | 82% |
| | 8 | 0.4013(10) | – | 0.83(13) | 0.10 | 76% | 0.4015(10) | – | -0.16(12) | 0.05 | 82% |
| | $\infty$ | 0.3985(13) | 0.473(88) | – | 0.21 | 65% | 0.3988(13) | 0.462(88) | – | 0.14 | 71% |
| $t'_1/t'_0$ | 3 | 0.4188(33) | – | 1.13(93) | 0.07 | 79% | 0.4187(33) | – | 0.29(92) | 0.07 | 79% |
| | 5 | 0.3911(13) | – | 0.93(22) | 0.03 | 86% | 0.3910(13) | – | -0.14(21) | 0.07 | 79% |
| | 8 | 0.38062(86) | – | 0.896(98) | 0.14 | 71% | 0.38083(85) | – | -0.274(94) | 0.07 | 78% |
| | $\infty$ | 0.3744(11) | 1.083(91) | – | 0.17 | 68% | 0.3747(11) | 1.069(91) | – | 0.09 | 76% |
| $w_0^2/t_0$ | 3 | 1.044(14) | – | -0.6(1.6) | 0.02 | 90% | 1.043(14) | – | -0.2(1.6) | 0.02 | 90% |
| | 5 | 1.085(11) | – | -0.62(70) | 0.01 | 91% | 1.085(11) | – | -0.24(70) | 0.01 | 93% |
| | 8 | 1.0976(66) | – | -0.47(31) | 0.13 | 72% | 1.0973(65) | – | -0.04(30) | 0.10 | 75% |
| | $\infty$ | 1.1067(77) | -0.51(14) | – | 0.02 | 90% | 1.1064(76) | -0.51(14) | – | 0.01 | 91% |
| $w_0'^2/t'_0$ | 3 | 1.044(14) | – | -0.6(1.6) | 0.02 | 90% | 1.043(14) | – | -0.2(1.6) | 0.02 | 90% |
| | 5 | 1.111(10) | – | -0.61(58) | 0.01 | 90% | 1.110(10) | – | -0.21(58) | 0.01 | 92% |
| | 8 | 1.1324(64) | – | -0.45(26) | 0.18 | 67% | 1.1321(63) | – | -0.02(26) | 0.15 | 70% |
| | $\infty$ | 1.1470(74) | -0.81(14) | – | 0.01 | 94% | 1.1468(73) | -0.81(13) | – | 0.01 | 95% |
| $t_0/t'_0$ | 3 | 1 | – | 0 | – | – | 1 | – | 0 | – | – |
| | 5 | 1.0898(49) | – | -0.05(28) | 0.01 | 98% | 1.0898(50) | – | -0.01(28) | 0.01 | 99% |
| | 8 | 1.1235(35) | – | -0.07(13) | 0.01 | 97% | 1.1234(35) | – | -0.01(13) | 0.01 | 98% |
| | $\infty$ | 1.1433(42) | -1.139(87) | – | 0.13 | 72% | 1.1432(42) | -1.138(87) | – | 0.12 | 73% |

Table 29: Continuum and large-$N$ limits and other best-fit parameters of scale ratios, with and without improvement of lattice artifacts. Data points at different values of $N$ were extrapolated to the continuum independently (see Eq. (46) in the text). Then, the continuum extrapolations were extrapolated to $N = \infty$ (see Eq. (47) in the text). All fits have one degree of freedom. For $N = 3$, primed and not primed scales are equal by definition.

## 3.2 Global fit strategy

| Global fit strategy | | | | | | | | | | |
|---|---|---|---|---|---|---|---|---|---|---|
| | Unimproved | | | | | Improved | | | | |
| Ratio | R | $C$ | $D$ | $\chi^2_{\text{red}}$ | $p$-value | R | $C$ | $D$ | $\chi^2_{\text{red}}$ | $p$-value |
| $t_1/t_0$ | 0.3985(10) | 0.492(34) | 0.83(11) | 0.29 | 94% | 0.3986(10) | 0.498(35) | -0.14(11) | 0.32 | 93% |
| $t'_1/t'_0$ | 0.37442(87) | 1.097(36) | 0.894(89) | 0.23 | 97% | 0.37439(87) | 1.124(36) | -0.259(85) | 0.43 | 86% |
| $w_0^2/t_0$ | 1.1070(66) | -0.520(63) | -0.50(28) | 0.03 | 100% | 1.1066(65) | -0.529(63) | -0.08(27) | 0.04 | 100% |
| $w_0'^2/t'_0$ | 1.1471(63) | -0.821(60) | -0.47(24) | 0.06 | 100% | 1.1468(63) | -0.829(60) | -0.05(23) | 0.07 | 100% |
| $t_0/t'_0$ | 1.1424(34) | -1.126(35) | -0.05(12) | 0.12 | 99% | 1.1425(34) | -1.130(35) | 0.00(12) | 0.14 | 99% |

Table 30: Best-fit parameters of the lattice-spacing-dependence of scale ratios, with and without improvement of lattice artifacts. Data points at all the values of $N$ were fitted together (see Eq. (48) in the text). All fits have 6 degrees of freedom.
